# Supplementary material for: Leveraging Public-Private Blockchain Interoperability for Closed Consortium Interfacing
Source: arXiv:2104.09801 source file (2021-04-20)
Supplement: Supplementary file 1 [file appendices.tex]

\appendix

\section{Brief Background on Blockchain and Smart Contracts}

\subsection{Smart Contracts Execution Flow}
\label{append:smartcontract}
%The idea of smart contracts goes back to 1997, which talks about enforcing and executing contracts with the help of software and hardware based protocols \cite{smartcontracts}.

%The fundamental functionality that blockchains provide is \textit{agreement} or \textit{consensus} among its participants. This consensus can be on a value, or on a set of instructions. Smart contracts are programs on which the blockchain network has consensus. 
%Additionally, each execution of the smart contract must also be agreed upon by the participants~\cite{cheng2019ekiden}. Thus, smart contracts have to be executed by all (or majority depending on the consensus requirement) the participants in the network taking part in the consensus process. The consensus criteria of smart contract execution brings two new considerations --
%\begin{enumerate}[(a)]
%\item  The exectution of the contract must be deterministic (so that consensus can be reached).
%\item If the contract acts on a state or value, then the blockchain must have consensus on that state or value too.
%\end{enumerate} 
%There are many smart contract execution platform including public Ethereum's quasi-Turing complete  \textit{Ethereum Virtual Machine} (EVM)~\cite{ethereum}, private Fabric's containerized smart contract engine which is decoupled from the consensus protocol~\cite{fabric}.

Although fundamentally, the execution of smart contracts are based on consensus on each execution result, there are two major different flavors of the flow of smart contract execution.
\begin{enumerate}[(a)]
\item \textbf{Order-Execute}: This is the traditional flow used in most blockchains like Ethereum, Hyperledger Burrow, etc., which involves three steps -- (i) reach to the consensus on the set of contract execution transactions and also their ordering, (ii) execute each of those transactions sequentially and deterministically, and (iii) update the state of each contract on the blockchain ledger according to their execution result.

\item \textbf{Execute-Order}: Here, the transactions are first simulated (executed) to find their results and corresponding change in the current blockchain state. Then these transaction results are ordered and the consensus is reached on them. Finally, the results are applied on the current state while rejecting conflicting transactions~\cite{fabric}. We discuss about conflicting transactions with an example later in this section.
\end{enumerate}
The execute-order method of processing smart contracts can have several advantages including parallel execution and ability to process non-deterministic transactions with no safety violation~\cite{fabric}. However, it can have performance limitations due to failed conflicting transactions which are executed in parallel and then ordered.

\textbf{Smart Contract execution flow:} Consider the simple counting contract as shown in Algorithm \ref{algo:contract}, which maintains a counter state from 0 to 99. The count can be changed by incrementing it through \textit{CallIncrement}, or doubling it through \textit{CallDouble} procedures.

\begin{algorithm}
	\caption{Counting Contract}\label{algo:contract}
	\begin{algorithmic}[1]
		\State State Variable: $count$
		\Procedure{Init}{}\Comment{Contract deployment}
		\State $count\gets 0$
		\EndProcedure
		
		\Procedure{CallIncrement}{}\Comment{Contract execution}
		\State $count\gets count + 1 \mod 100$
		\EndProcedure
		
		\Procedure{CallDouble}{}\Comment{Contract execution}
		\State $count\gets count \times 2 \mod 100$
		\EndProcedure
	\end{algorithmic}
\end{algorithm}

The first step is to deploy or install and initialize the contract in the blockchain. This step involves agreement on (a) the contract program (the instructions), as well as (b) on the initial state of the contract, that is the \textit{count} variable in this case. This initial state is decided through the \textit{Init} procedure. Thus the blockchain participants agree on the initial value of \textit{count} variable to $0$.

After deployment, any participant can execute the contract. Such executions are done by \textit{transactions}, each of which denote that a participant is executing the contract once. Transactions include which procedure of the contract is being called, by which participant or contract, and also the arguments passed by the caller. Later we discuss what happens if two participants fire two transactions simultaneously. Let the two transactions be of different types, one \textit{CallIncrement} ($\mathcal{I}$) and another \textit{CallDouble} ($\mathcal{D}$).

\textbf{Order-Execute flow:} First the transactions and their order are agreed upon through the consensus process. The order can depend on various parameters such as transaction fees in Bitcoin and Ethereum. Thus, the order can be $\mathcal{I,D}$ or $\mathcal{D,I}$. After consensus, the transactions are executed by each participant sequentially, resulting in the new \textit{count} value to be $2$ or $1$ respectively in the two orderings. Finally the state of the blockchain, which is the current value of the \textit{count} variable, is updated with this new value. The subsequent transaction executions are applied on this updated state.

\textbf{Execute-Order flow: } The transactions are first executed by the participant on the current state (say version $v_{t-1}$ ) to find the result (updated state $v_{t}$). This updated state, along with the version number of the last state is sent out as the transaction for consensus. Thus, if $\mathcal{I}$ is executed first, then the value of $count$ is calculated as $1$, and this is sent for consensus and ordering. After the consensus is reached the state is updated with $count=1 ~(version~v_{t})$. After this process is complete, if $\mathcal{D}$ is executed, then it acts on the updated state ($count=1$ in $v_{t}$) and after the execution finishes, the new state becomes $count=2$ in version $v_{t+1}$. Similarly, if first $\mathcal{D}$ and then $\mathcal{I}$ were executed, then the final state would have been $count=1$.

However, the problem comes when both the transactions are simulated in parallel by the two participants to find the updated state before sending it for consensus. On the initial state of $count=0$ in $v_{t-1}$, simulating $\mathcal{I}$ results in $count=1$, while $\mathcal{D}$ results in $count=0$. Then both of these updated states are sent for consensus. Simply applying these transactions one after another can clearly result in incorrect state. For example, if the order is agreed as $\mathcal{I,D}$, the correct resulting state should be $count=2$. Whereas, by applying $count=1$ first and then $count=0$ next from the updated states of the transactions, the final state becomes $count=0$, which is incorrect. Therefore, in order to prevent such conflicting transactions acting on the same state, the version of the state on which the transaction acts is checked. This is called \textit{Multiversion concurrency control}~\cite{mvcc}, used in databases. Thus the two (or more) parallel transactions both simulated on $v_{t}$ are conflicting, and thus only one of them can be committed and the rest will fail. These failed transactions will need to be executed again on the updated state.
