# Supplementary material for: Leveraging Public-Private Blockchain Interoperability for Closed Consortium Interfacing
Source: arXiv:2104.09801 source file (2021-04-20)
Supplement: Supplementary file 2 [file appendices_discarded.tex]

\subsection{Choice of a public blockchain platform} 
\label{append:pubchain}
\textit{CollabCloud} architecture is independent of the underlying public blockchain platform used, and thus, it is a pluggable component. Primarily, the choice depends on the consensus protocol used by the blockchain platform, which is reponsible for providing \textit{Federation Interface Safety} and \textit{Federation Interface Liveness}. Thus, the protocols must be byzantine fault tolerant, and it must be resilient against sybil attacks. 
This ensures that all the participating CSPs get the same set of user requests and in the same order as long as the network satisfies the assumptions of the underlying consensus protocol in use.
\textit{CollabCloud} also requires quick transaction commitment times since it directly affects the quality of service of the end-users. The faster the user requests get committed in the public blockchain, the quicker the CSPs can start scheduling and VM provisioning.

\textbf{Proof of Work} (PoW) consensus based blockchains like Bitcoin, Litecoin, Ethereum etc., account for the majority of market capitalization in digital cryptocurrencies \footnote{\url{https://coinmarketcap.com/}}. The safety property of this consensus protocol holds with the assumption that no entity (single or colluded) has more than 50\% of the processing power in the network~\cite{gervais2016security}. However, there have been other attacks like ``selfish mining''~\cite{selfishmining}, ``eclipse attacks''~\cite{heilman2015eclipse}, etc. which can further compromise the safety of the network. In terms of liveness, PoW mines all the transactions eventually as long as the network is partially synchronous and under the control of honest miners (safety conditions are satisfied). The transaction fees also govern how fast a transaction will be committed~\cite{kasahara2016effect}. The rate of producing new blocks has a trade-off with the safety of the blockchain, with stale block rate of 0.41\% in Bitcoin compared to 6.8\% in Ethereum due to the faster confirmation time in the later \cite{gervais2016security}. As a result, the transaction rates of these blockchains are slower ( < 100 transactions per second ) compared to other alternatives \cite{byzcoin}.

\textbf{Proof of Stake} (PoS) consensus protocols have been developed to reduce the resource consumption required for the consensus process in case of PoW, and they also offer better transaction confirmation latency~\cite{algorand, ouroboros}. The condition under which PoS blockchains maintain the safety property is that more than two thirds ($> \frac{2}{3}$) of the stake (for example cryptocurrency) is owned by the honest users. Based on this stake, a leader or a committee is elected which is responsible for mining blocks \cite{algorand}. For ensuring the liveness property, these blockchains depend on certain practical assumptions like network reachability, strong network synchrony~\cite{algorand}, elected committee members participate in the consensus process, and stakeholders do not remain offline for a long period of time~\cite{ouroboros}. The transaction throughput and latency of PoS blockchains are much improved when compared to the PoW ones, with Algorand claiming 125$\times$ throughput of Bitcoin \cite{algorand}.

\textbf{BFT Based} protocols have also recently gained much attention with Bitcoin-NG~\cite{bitcoin-ng} and Byzcoin~\cite{byzcoin}. These blockchains use traditional BFT protocols such as PBFT \cite{pbft} in order to achieve consensus in a close committee which is elected and changed over time through PoW. Thus, PoW is used only for electing committees, while the transaction blocks can be generated quickly by the committees using BFT protocols. The safety assumption of such consensus protocols is that the byzantine nodes should have less than $\frac{1}{4}$ of the system’s total hash power at any time. For liveness, they rely on the weak synchrony property of the network~\cite{byzcoin}. Because of the decoupling of committee/leader election using PoW and mining blocks using BFT protocols, these protocols achieve a very high throughput (around 1000 transactions per second in Byzcoin).

Apart from PoW, PoS and BFT based protocols there are other consensus protocols such as Proof-of-Useful-Work \cite{zhang2017rem}, Proof-of-Elapsed-Time \cite{chen2017security} etc. are also discussed in the literature.

\subsection{Determination of VM pricing in a federation}
\label{appen:pricing}
Several works in the existing literature focus on the pricing aspect in cloud federations~\cite{cardellini2016game, kaewpuang2013cooperative, samaan2013novel}, as well as revenue sharing~\cite{el2014federation, hassan2015socially}. They have considered multi-cloud resource exchange-based architectures as well as broker-based architectures. The pricing model can depend on various factors like (i) how cooperative or competitive the environment is, (ii) is there any provision for profit sharing, and (iii) does all the providers have some unique offering or are they competing for pricing of same kind of resources. Moreover, the pricing policy also depends on whether its goal is to provide the best pricing to the end users or to maximize the profit for the federation, or a balance between the two. The pricing thus also depends on the scheduling policy of the federation. 

As an example, a simple pricing policy that will ensure profit for the federation participants, irrespective of the scheduling and revenue sharing policy is described below. 

For each VM configuration type, the federation catalog pricing for that VM is set to be greater than the maximum cost for the same configuration by any CSP in the federation. It can be represented as,
\begin{equation*}
\scriptsize
\begin{aligned}
catalogprice(\mathcal{V}_{j}) > max~( \mathcal{O}.c~ \forall~\{~O ~\in~ \bigcup\limits_{\mathcal{C}_i \in \mathcal{F}}  \mathbb{O}^{\mathcal{C}_i} ~|~O.\mathcal{V}=\mathcal{V}_{j},~O.k>0 \})\\
\forall \mathcal{V}_{j} \in \mathbb{C}
\end{aligned}
\end{equation*}

This will ensure that each type of VM provisioning will be profitable for each CSP in the federation. However with such pricing, it might be too high for the end users. As an alternative, a lower user friendly pricing might be preferred which can be adjusted according to demand when the cheaper offerings are sold out. For this the catalog price of each VM configuration can be set to be just higher than the lowest cost offering by any CSP for that configuration, which is still free (available). Therefore,
\begin{equation*}
\scriptsize
\begin{aligned}
catalogprice(\mathcal{V}_{j}) > min~( \mathcal{O}.c~ \forall~\{~O ~\in~ \bigcup\limits_{\mathcal{C}_i \in \mathcal{F}}  \mathbb{O}^{\mathcal{C}_i} ~|~O.\mathcal{V}=\mathcal{V}_{j},~O.k>0 \})\\
\forall \mathcal{V}_{j} \in \mathbb{C}
\end{aligned}
\end{equation*}
This price can be later adjusted as resources get exhausted with demand.

More comprehensive pricing policies based on game theoretic analysis can be applied with suitable revenue sharing models, which are out of scope of this work.

%\section{Choice of permissioned blockchain platform}
\subsection{Choice of a private blockchain platform}
\label{appen:private}
\textit{CollabCloud} is independent of the private blockchain platform used, and it is a pluggable component. The choice of the private blockchain depends primarily on the consensus protocol used by it. Different consensus protocols affect the conditions under which the blockchain ensures safety and liveness in the presence of Byzantine faults. It also impacts the latency of processing each transaction affecting the performance of the overall system. We discuss some of the popular pemissioned blockchain pltforms and their safety and liveliness assumptions.

\textbf{Hyperledger Fabric} supports multiple consensus protocols as a pluggable component of the ordering service \cite{fabric}. This includes crash fault tolerant orderer or a Byzantine fault tolerant order based on BFT-SMaRt protocol \cite{sousa2018byzantine}. The safety property of BFT-SMaRt holds under the assumption that the number of faulty participants is less than one third ($< \frac{1}{3}$) of the total number of participants in the blockchain. For liveness, BFT-SMaRt requires that the network satisfies eventually synchronous property \cite{bftsmart}. Hyperledger fabric follows execute-order flow for transactions and reports transaction throughput of more than 2000 per second \cite{sousa2018byzantine}.

\textbf{Hyperledger Burrow} is a private blockchain platform based on the Tendermint consensus protocol \cite{tendermint}. Similar to PBFT and BFT-SMaRt, Tendermint protocol's safety property requires that less than one third of the total participants in the system are Byzantine faulty. If the safety condition is satisfied, then with the assumption that the network has partial synchrony property, Tendermint also satisfies liveness.

\textbf{Hyperledger Iroha} is a distributed ledger for decentralized identity, and it uses YAC consensus protocol \cite{yac} which ensure safety and liveness under assumpations similar to PBFT \cite{pbft}.

\textbf{Hyperledger Indy} uses the Plenum consensus protocol\footnote{\url{https://github.com/hyperledger/indy-plenum/wiki}}, which is an implementation of RBFT \cite{aublin2013rbft}. RBFT is based on the PBFT protocol, with parallel PBFT flows for more robustness. It has the same assumption for safety property that less than one third of total nodes in the system are Byzantine faulty. For liveness it relies on the assumption of an asynchronous network with synchronous intervals, during which
messages are delivered within an unknown bounded delay. With a lab network setup of 8 nodes, RBFT claims throughput of upto 5000 requests per second of size 4KB each.

\section{\textit{CollabCloud} Implementation Details}
\label{appen:impl}
For ensuring the reproducibility of our implementation of \textit{CollabCloud}, here we give the details about the toolboxes used in the implementation along with the process flow during execution of an end-user request.   
\subsection{Implementation Specifications}
Starting from the top of the architecture, the \textit{CollabCloud Client} provides a GUI, through which users can query and transact with  \textit{CollabCloud Unified Interface}. The frontend GUI is provided by a web interface with \texttt{Express.js}\footnote{\url{https://expressjs.com/}} server build within the client. The client uses \texttt{Web3.js (v1.2.1)}\footnote{\url{https://web3js.readthedocs.io/en/v1.2.1/}} for interaction with Ethereum node. We have used the GO language implementation of Ethereum client, \texttt{Geth:} 1.9.3\footnote{\url{https://github.com/ethereum/go-ethereum}}. The client also runs an event listener which monitors transactions on Ethereum and identifies any changes in the federation information or response to any user request. In case of federation information update, the same is reflected in the web interface. Any information from the federation is validated by verifying the BLS multi-signature against the public keys of the CSPs. For all BLS signature operations we use the \texttt{PBC Library}\footnote{\url{https://crypto.stanford.edu/pbc/}}.

In the federation side, each CSP has has several components to interact with the public blockchain, participate in the private blockhain network, collect multi-signatures and provision infrastructure as VMs. 
%Each CSP has an Ethereum interface for capturing and monitoring transactions on it, and executing new transactions. This interface is again implemented using \texttt{Web3.js} and \texttt{Truffle}.
The \textit{CollabCloud CSP Interface} acts as a bridge between the public blockchain (Ethereum) and the private blockchain (Fabric and Burrow). The heart of the CollabCloud CSP Interface is implemented as a service which handles 4-way coordination between (i) the public blockchain, (ii) the private blockchain, (iii) the multi-signature collector, and (iv) the CSP's resource provisioning service. This coordinator is implemented using Python and \texttt{Flask}\footnote{\url{https://flask.palletsprojects.com/}} which exposes APIs for interfacing with the other components of \textit{CollabCloud}.

In order to interact with public blockchain (Ethereum), \textit{CollabCloud CSP Interface} provides event listeners for monitoring user requests, and it also lets CSPs to execute transactions on \textit{CollabCloud Unified Interface} smart contracts. The event listeners and smart contract execution is handled by \texttt{Web3.js} interacting with \texttt{Geth} client. 

For communication with the public blockchain, \textit{CollabCloud} provides a REST API endpoint which can be used by the CSPs through the \texttt{Flask} based coordinator. In order to interface with Hyperledger Fabric, the \texttt{Fabric Node.js SDK} is used. This SDK along with \texttt{Express.js} provides the API endpoint implementation. For Hyperledger Burrow, the \texttt{Burrow JS SDK} is used along with \texttt{Express.js}.

The \textit{Multi-signature Collector} coordinates the collection of BLS short signatures off chain by directly requesting each CSP. It is assumed that during normal situations, each CSP that participated in the consensus process will sign the transaction. In case a CSP goes rogue and does not sign within a given timeout, a backup smart contract for collection of signatures through private blockchain is executed. This is important to detect and keep in check any malicious behaviors from the participating CSPs. We use \texttt{PBC Library} for signing and verification purposes.

Finally, we had two separate implementations of the \textit{Fair Request Scheduling} smart contract, one for Fabric and another for Burrow. For Fabric, the contract is implemented in Go programming language. For Burrow the same is done using Solidity language.

\color{red}
\subsection{Components of interface}

CollabCloud provides \textit{Brokerless Federation Interface} over a public blockchain using two components -- (i) \textit{\textbf{CollabCloud Client}} which is used by the end-users to interact with the federation, and (ii) \textit{\textbf{CollabCloud Unified Interface}} which are smart contracts that are used by both \textit{CollabCloud Client} and the CSPs participating in the federation.
\subsection{\textit{CollabCloud} Client}
The \textit{CollabCloud Client} is an application which is used by the individual end-users. This acts as an interface between the users and the \textit{CollabCloud Unified Interface} of the public blockchain. The application is responsible for creating an account (wallet) on the blockchain and generating a public-private key pair (public key: $\mathcal{P}_{\mathcal{U}}$, secret key: $\mathcal{S}_{\mathcal{U}}$). 
%which is used for providing access to the federation resources. \textit{CollabCloud Client} creates a wallet (account) for the end-user to access the permissionless blockchain. This creates a cryptographic key pair for the user . 
The public key of each user also acts as its identifier and allows the secure transfer of resources through the blockchain (Section \ref{subsec:secureinfotransfer}). Through this client, the end-users can query for information like catalog of resources, pricing, SLA information, etc. Further, the users can choose a resource specification and request it from the federation. 
%When a request is granted, the access information is given to the user, and the payment process is handled by \textit{CollabCloud Client}. The client also performs a very important role of verifying the authenticity of information obtained from the blockchain, as discussed in Sec.~\ref{subsec:secureinfotransfer} in details.
\subsection{\textit{CollabCloud} Unified Interface}
\textit{CollabCloud Unified Interface} consists of smart contracts deployed on the public blockchain which are responsible for handling the logic of the unified interface between the end-users and the CSPs. 
%These include smart contracts for (a) requesting resources (\textit{Resource Request}), (b) getting resources in response of the requests (\textit{Resource Provisioning}), (c) querying federation information like SLA, participating CSP details, etc. (\textit{Information Management}), and (d) querying catalog and pricing details (\textit{Catalog Management}). Among these, the \textit{Resource Request} contract is responsible for generating the transactions at the public blockchain interface, and the remaining three smart contracts provide necessary information to the end-users and thus are read-only to the end-users. 
The details follow. 
\subsubsection{Resource Request Contract}
This smart contract allows the end-users to request for resources. A user-request is defined as a four-tuple: $\mathcal{R} = \{ \mathcal{R}_{id}, \mathcal{P}_{\mathcal{U}},  \mathcal{V}_{j}, \mathcal{D} \}$, where $\mathcal{R}_{id}$ is the unique identifier of the user request, $\mathcal{P}_{\mathcal{U}}$ is the public key of the end-user making the request, $\mathcal{V}_{j} \in \mathbb{C}$ is the VM configuration selected from the catalog $\mathbb{C}$, and $\mathcal{D}$ is the duration for which the VM is requested. This request $\mathcal{R}$ is posted by the end-user through the \textit{CollabCloud Client}.
Once the users post their requests, this contract is executed to propose a transaction in a new block for the public blockchain network. In a public blockchain network, the miners mine a new block from the set of transactions posted from the end-users as well as the CSPs. The task of the miners is to ensure an ordering of the posted transactions based on the business logic of the network, and then execute an open consensus mechanism, like PoW, PoS, etc. (Appendix \ref{append:pubchain}), so that the network as-a-whole agrees on each proposed block. In the \textit{CollabCloud} federation interface, every user request is considered as a transaction for the public blockchain network. Although any business logic can be applied for ordering the requests, in our implementation, we order the transactions based on the decreasing amount of the transaction fee. This transaction fee is an amount proportional to the requested resource capacity, which every user pays against each resource requests\footnote{An idea similar to the credit card validation/pre-authentication during resource requests over popular CSPs, like Amazon Web Services or Microsoft Azure.}; this is a pre-validation token which is adjusted during the billing based on the actual resource usage. Once the user requests are committed in the public blockchain, the CSPs can access the resource requests details. Each CSP continuously monitors the public blockchain for a new \textit{Resource Request Contract} transactions through an event listener; once such an event gets triggered, the CSPs collectively execute a resource scheduling mechanism, as discussed in Section~\ref{sec:collaboration}.

\subsubsection{User Read-only Contracts}
The rest of the smart contracts are read-only for the end-users, where the end-users obtain federation and resource allocation related information. These contracts are updated by the CSPs through collective consensus via three other smart contracts running over the private blockchain, as discussed in Section~\ref{sec:collaboration}. 
%As we mentioned earlier, transferring the consensus information from the private blockchain to the public blockchain is done through a secure information transfer protocol which is discussed in Sec.~\ref{subsec:secureinfotransfer}. 
The descriptions of these smart contracts follow.

\textbf{Resource Provisioning Contract:} 
This smart contract allows the CSPs to securely give access of the resources to the end users. The primary objective of this smart contract is to ensure that the allocated resource is an outcome of the collective decision of the federation, and is not from an adversarial CSP. This is particularly important because anyone can try to post an information over the public blockchain because it does not require a pre-authentication of the end-users. A signed encrypted token containing the resource access details are posted on the public blockchain network; the signing procedure is described in details in the \textit{Secure Resource Transfer} sub-module (Section~\ref{subsec:secureresourcetransfer}). This token is encrypted by the public key of the user who originally requested for the resource; therefore only the valid end-user can access it. 

%It is important for a cloud federation to be easily accessible to its users. The complexity of the decentralized architecture of \textit{CollabCloud} should be transparent to the end users, and this is made possible by the \textit{CollabCloud Client}. It provides the users a familiar interface through which they can query the catalog, read the SLA, pricing policies etc., request resources and get access to them. All these functions are provided by the \textit{CollabCloud Client} with the help of \textit{CollabCloud Unified Interface}. The unified interface consist of smart contracts that implement the functionalities required to interact with the federation in a permissionless blockchain. The interface contracts are not only used by the end-users, but also by the CSPs and thus acts as the point of contact between the two groups. The contracts include - 

\textbf{Information Management Contract:} 
This smart contract is used for  querying and updating the information of the federation. This includes a list of the CSPs participating in the federation $\mathcal{F} = \{ \mathcal{C}_{1}, \mathcal{C}_{2}, . . , \mathcal{C}_{n} \}$, and their business information. For example, this should include the name of each participating CSP, their company name and company registration detail, address, contact information, their individual privacy policies etc.. Apart from that each CSP will list its public key $\mathcal{P}_{\mathcal{C}_{i}}$ which also acts as their unique identifier, and the FLA containing the information about the joining date of a CSP in the federation, a copy of the federation joining contract digitally signed by all preceding CSPs and the joining CSP, the expiry date of the contract and the terms to ensure service quality by each such CSP. 
%\notesc{Here you need to give the details, or examples. like what do you mean by business information, what is the FLA.} 
A transaction to this contract is executed by the \textit{Information Updation Contract} as discussed in Section~\ref{subsec:infoupdate}. 

%This smart contract 
%In order to update information of the federation, the consensus of all the participants is required. As a result, no individual CSP can make a valid transaction to change the information through \textit{Information Management Contract}. For a transaction to be valid, it must be collectively signed by majority of the participants of the federation. This process is carried out by the \textit{Information Updation Contract} in the \textit{CollabCloud Collaboration Contracts} through the persmissioned blockchain which is explained in detail in the following section.

\textbf{Catalog Management Contract:} 
This smart contract is used for updating and querying the catalog of the federation. The CSPs participating in the federation may provide different VMs with different specifications. A CSP $\mathcal{C}_i$ can support certain VM configurations which are represented by $\mathbb{V}^{\mathcal{C}_i} = \{ \mathcal{V}_1,\mathcal{V}_2, . . , \mathcal{V}_m \}$. Each $\mathcal{V}$ is a distinct four tuple: $\{ \mathcal{CPU}, \mathcal{MEM}, \mathcal{PS}, \mathcal{LOC} \}$, where $\mathcal{CPU}$ is the number of virtual CPU cores in the VM, $\mathcal{MEM}$ is the memory of the VM in GB, $\mathcal{PS}$ is the persistent storage associated with the VM, and $\mathcal{LOC}$ is the location of the data center where the VM will be placed. Thus the catalog of the federation is the union of all such VM configurations being offered by the individual CSPs, represented as $\mathbb{C} = \bigcup\limits_{\mathcal{C}_i \in \mathcal{F}}  \mathbb{V}^{\mathcal{C}_i}$. A transaction to this contract is executed by the \textit{Catalog Updation Contract} as discussed in Section~\ref{subsec:catupdate}. 

%The CSPs use \textit{CollabCloud Unifed Interface} to monitor user requests, update the catalog and information of the federation, and giving users the access to the  provisioned resources. Each CSP continuously monitor the blockchain for new \textit{Resource Request Contract} transactions through an event listener. Whenever a new request arrives, the CSPs collaborate to schedule the same. After the request is scheduled and the resource is provisioned, the CSPs use the transfer the credentials securely to the end-users.

\subsubsection{Federation Interface Safety and Liveness}
The safety and liveness criteria of the federation interface depends on the choice of the public blockchain platform and the corresponding consensus mechanism used for smart contracts. We discuss a comparison of various public blockchain platforms in terms of their safety and liveness in Appendix~\ref{append:pubchain}.

\color{blue}

\section{Brokerless Collaboration}
\label{sec:brokerlesscollaboration}
\textit{CollabCloud} provides \textit{Brokerless Collaboration} over a private blockchain platform using three components -- (i) \textit{\textbf{CollabCloud CSP Interface}} which is used by the CSPs to participate in the federation by connecting to both the public and the private blockcahins,  (ii) \textit{\textbf{CollabCloud Collaboration Contracts}} which are smart contracts of the private blockchain used by the CSPs participating in the federation, and (iii) \textit{\textbf{\textbf{Multi-signature Collector}}} which allows the end-users to verify the authenticity of the federation responses.

\subsection{\textit{CollabCloud} CSP Interface}
The CSPs of \textit{CollabCloud} must interact with both the public blockchain for receiving user requests and interacting with the end-users, as well as the private blockchain for coordinating with other CSPs. This is facilitated by the \textit{CollabCloud CSP Interface} that provides the CSPs the interface through which they can execute the contracts under the \textit{CollabCloud Unified Interface} in the public blockchain, as well as can listen for transaction events for responding to user requests. It also provides the interface to the private blockchain and enables the CSPs to execute transactions through \textit{CollabCloud Collaboration Contracts}. The result of the \textit{CollabCloud Collaboration Contracts} can directly trigger a transaction in the public blockchain through the \textit{CollabCloud CSP Interface}, as we discuss later. Thus \textit{CollabCloud CSP Interface} establishes a bridge between the public blockchain and the private blockchain. The most important role while providing this bridge is passing the consensus of the public blockchain to the private blockchain. A request received through the public blockchain cannot be processed immediately as an adversarial CSP might start processing a request which might have not came through the federation interface. Therefore consensus on each request should be reached among the CSPs, in order to process it further.

\textbf{Consensus Propagation From the Public Blockchain to the Private Blockchain:}
The federation should execute the scheduling of a user-request only when it passes through the consensus of the public blockchain, ensuring that a malicious CSP cannot collude the federation by triggering the scheduling of an out-of-federation user request. The \textit{CollabCloud CSP Interface} of each CSP listens for new transactions of the \textit{Resource Request} contract. Whenever a new resource request is committed (consensus is reached in the public blockchain), the user-request $\mathcal{R}$ along with its sequence number in the public blockchain is used to start a \textit{Propagation Contract}. The task of the \textit{Propagation Contract} is to collect verification votes from CSPs for each user-request. When it is executed for the first time by any CSP, the vote count is registered as 1, and the signed vote of that CSP is committed. As other CSPs also get the user-request through the event listener of the public blockchain, they also execute the \textit{Propagation Contract} for it which adds their signed votes. Thus, the number of votes go up until it reaches greater than two third of the number of CSPs ($votes > \frac{2}{3} |\mathcal{F}|$). At this point, the user-request is marked as approved and  \textit{Propagation Contract} executes \textit{Fair Request Scheduling} contract discussed in Section~\ref{fairscheduling}. It is to be noted that each execution of \textit{Propagation Contract} and thus each vote also goes through the consensus process of the private blockchain.

\subsection{\textit{CollabCloud} Collaboration Contracts}
\textit{CollabCloud Collaboration Contracts} facilitate the scheduling of user requests, the updation of federation information, and the updation of individual CSP catalogs. It includes three contracts as follows.

\subsubsection{Information Updation Contract} 
\label{subsec:infoupdate}
This smart contact enables the participating CSPs to update their own details, as well as the information of the federation as a whole. It also enables new CSPs to join the federation. Whenever a new CSP joins the federation or an existing CSP wants to update its information, it generates a transaction to the private blockchain network that needs to be executed through this contract. In order to execute a valid transaction through this contract, a CSP must aggregate endorsements (signatures) from majority of the participating CSPs in the form of multi-signature as described in Section~\ref{subsec:secureinfotransfer}. 
%This ensures that the federation information can only be updated when a consensus is reached on the acceptance of the information by majority of the CSPs.

It can be noted that the joining of a new CSP can be based upon the business logic of the federation. For example, the federation may accept a new CSP only when it conforms to the FLA. In this case, a CSP endorse (sign) the transaction only if the transaction meets the FLA criteria. On successful execution of this contract (upon consensus), it triggers an update to the \textit{Information Management Contract} over the public blockchain through the \textit{CollabCloud CSP Interface}. 

\subsubsection{Catalog Updation Contract} 
\label{subsec:catupdate}
This allows a CSP to update its contribution of resources to the federation. Accordingly, the catalog of the federation is updated in the public blockchain and the contribution of the CSP is evaluated in the private blockchain for fair scheduling of user-requests. Similar to the catalog which is a set of VM configurations, the contribtion of each CSP $\mathcal{C}_i$ is a set of \textit{VM offerings}, denoted by $\mathbb{O}^{\mathcal{C}_{i}} = \{ \mathcal{O}_1, \mathcal{O}_2 .. \mathcal{O}_m \}$. A \textit{VM offering} is defined as a three-tuple: $\mathcal{O} = \{\mathcal{V},k,c\}$, where $\mathcal{V}$ denotes a VM configuration as defined previously, $k$ denotes the quantity of the VMs of the particular configuration the CSP can offer, and $c$ denotes the expected pricing of that VM type. 

Similar to the \textit{Information Updation Contract}, this contract also uses a business logic to decide the federation pricing for different VM types, and the consensus is reached on that based on the majority endorsements. This business logic for catalog preparation and catalog pricing depends on the federation; although the details is out of scope for this paper, we discuss a possible example scenario in Appendix~\ref{appen:pricing}.  
%The \textit{Catalog Updation Contract} takes input a \textit{VM offering}, and the transaction requires only the signature of the CSP executing it.

\subsubsection{Fair Request Scheduling Contract}
\label{fairscheduling}
This smart contract provides a fair scheduling of the end-user requests among the CSPs. Once a resource request is committed in the public blockchain, and the same is approved by the \textit{Propagation Contract} of \textit{CollabCloud CSP Interface}, the \textit{Fair Request Scheduling Contract} is triggered. The objective of this contract is to execute a deterministic procedure to decide which among the CSPs should cater to the request, based on the statistics available in the public blockchain through the \textit{Information Updation Contract} and \textit{Catalog Updation Contract}. The exact algorithm for fair scheduling is based on the business logic of the federation; we provide a sample scheduling algorithm and is performance in Appendix~\ref{appen:fairschedule}. \textit{CollabCloud} design is flexible to allow any scheduling algorithm provided that it is deterministic and the result is verifiable by all the participating CSPs ensuring a consensus in the system. To ensure this, following constraints need to be satisfied. 
\begin{enumerate}
	\item All the inputs to the algorithm should be based on the information available over either the public blockchain network or the private blockchain network or both. 
	\item The output of the algorithm must be deterministic.  
\end{enumerate}
The above constraints ensure that the output of the algorithm is verifiable by all the participating CSPs as all the CSPs get the same view of the system from the two blockchains. Typically, the CSPs verify the output of the algorithm to reach into a consensus over the private blockchain network. A private blockchain typically uses a BFT-based consensus mechanism (see Appendix~\ref{appen:private} for details) which relies on the $\tfrac{2}{3}$ of the total voting power from the participants~\cite{dwork1988consensus}. Through the \textit{Fair Request Scheduling} contract, one CSP is selected which will serve the request. This selected CSP performs VM placement according to its own placement policies. Once the VM is provisioned, the CSP enables user access by secure resource transfer scheme as discussed in Section~\ref{subsec:secureresourcetransfer}.  
